# Supplementary material for: ADEV: Sound Automatic Differentiation of Expected Values of Probabilistic Programs
Source: arXiv:2212.06386 source file (2022-12-13)
Supplement: Supplementary file 1 [file modularity-and-new-primitives.tex]

\section{Modularity of ADEV: adding new correct primitives to the language}

ADEV is quite flexible and modular. 
To show this, we add several new stochastic primitives that encompass various known distributions of various complexity from the literature, using several different gradient estimation strategies.  

\subsection{Simple REPARAM-like primitives}

If we have access to an analytic version of the inverse Cumulative Distributive Function (CDF) of a distribution and if it is differentiable, we can use it as a reparametrization for the REPARAM method. These are called inversion methods. Polar transforms and one-liners are two instances of this method. For univariate distributions, one can also obtain an alternative expression for the gradient using the CDF directly.
Let $x=g(\epsilon; \theta)=F^{-1}(\epsilon;\theta)$ where $F$ is the CDF and $\epsilon\sim \sample$. Then, using the that that the density $p(x,\theta)$ is the derivative of the CDF, we have \[
\grad_\theta x=-\frac{\grad_\theta F(x;\theta)}{p(x;\theta)}
\]
This is the implicit differentiation method. Using these, we can add the following primitives \cite{figurnov2018implicit, jankowiak2018pathwise, mohamed2020monte}:

\begin{itemize}
    \item multivariate Gaussian: $\normalreparam:\RR^n\times \RR^{n^2}\to \pmonad \RR^n$ is the simple generalization of the univariate case by doing $\epsilon\sim \mathcal{N}(0,I); z=\mu+L\epsilon;return~z$ with $LL^T=\Sigma$.
    \item Gamma: $\gammareparam:\posreal\times\posreal\to \pmonad\RR$ by forward-mode AD to a numerical method computing the value of the CDF.
    \item Dirichlet: $\dirichletreparam:\posreal^{K+2}\to \pmonad\RR^{K+2}$ can be obtained as $\dirichletreparam(\alpha_1,\ldots,\alpha_{K+2})=z_i\sim \gammareparam(\alpha_i,1);\return~(\frac{z_1}{\sum_j z_j},\ldots,\frac{z_{K+2}}{\sum_j z_j})$
    %\item Exponential: can be obtained as a one-liner or using the above.
    \item Beta: $\betareparam: \posreal\times\posreal\to \pmonad \RR$ can be obtained as $\betareparam(\alpha,\beta)= z_1\sim \gammareparam(\alpha,1);z_2\sim \gammareparam(1,\beta);\return~\frac{z_1}{z_1+z_2} $
    %\item von Mises distribution is a maximum entropy distribution on a circle with the density function $vonMises(z~|~\mu,\kappa)=\frac{}{}$  \cite{figurnov2018implicit}
    %item mixture distributions \cite{figurnov2018implicit}
    \item Student-t: $\studenttreparam:\posreal\to \pmonad \RR$ can be obtained as $\studenttreparam(\nu)=\sigma \sim \gammareparam(\frac{\nu}{2},\frac{\nu}{2}); z\sim \normalreparam(0,\sigma^2);\return~ z$
\end{itemize}

Importantly, the key argument above will be the main component in showing the correctness of these primitives in ADEV.

% \subsection{Derivative generalisations:  smoothed perturbation analysis }

% not really getting it. These are old papers from the 90s that are a bit hard to read now.

\subsection{Measure valued gradients estimators (weak derivative method, measure-valued derivative)}

The derivative $\grad_{\theta_i}p(x;\theta)$ of a density $p(x;\theta)$ is itself not a density but we can always decompose into a difference of two densities.
\[\grad_{\theta_i}p(x;\theta) = c^+_{\theta_i}p^+(x;\theta)-c^-_{\theta_i}p^-(x;\theta)\]
But we can in fact show that $c^+_{\theta_i}=c^-_{\theta_i}$ and therefore $\grad_{\theta_i}p(x;\theta)$ can be represented as a triple $(c_{\theta_i},p^+,p^-)$, and is referred to as the (i-th) weak derivative of $p(x;\theta)$.

With this, we can derive weak derivatives \cite{mohamed2020monte} and therefore new estimators for a variety of probability measures, which intuitively compute the gradient using a weighted difference of two expectations. We recap some known results in Figure~\ref{fig:weak-derivatives}, which can all be added in ADEV.
TODO: say how more precisely.

\begin{figure}
    \centering
\begin{tabular}{l|c|c|c}
\hline
    Distribution $p(x;\theta)$ & Constant $c_\theta$ & Positive part $p^+(x)$ & Negative part $p^-(x)$  \\ \hline
    Bernoulli($\theta$) & 1 & $\delta_1$ & $\delta_0$ \\
    Poisson($\theta$) & 1 & $\mathcal{P}(\theta)+1$ & $\mathcal{P}(\theta)$ \\
    Normal($\theta,\sigma^2$) & $\frac{1}{\sigma\sqrt{2\pi}}$ & $\theta+\sigma\mathcal{W}(2,0.5)$ & $\theta-\sigma\mathcal{W}(2,0.5)$ \\
    Normal($\mu,\theta^2$) & $\frac{1}{\theta}$ & $\mathcal{M}(\mu,\theta^2)$ & $\mathcal{N}(\mu,\theta^2)$ \\
    Exponential($\theta$) &  $\frac{1}{\theta}$ & $\mathcal{E}(\theta)$ & $\theta^{-1}\mathcal{E}r(2)$ \\
    Gamma($a,\theta$) & $\frac{a}{\theta}$ & $\mathcal{G}(a,\theta)$ & $\mathcal{G}(a+1,\theta)$  \\
    Weibull($\alpha,\theta$) &  $\frac{1}{\theta}$ & $\mathcal{W}(\alpha,\theta)$ & $\mathcal{G}(2,\theta)^{\frac{1}{\alpha}}$ \\
    \hline
\end{tabular}
  \caption{Weak derivatives triples. We use $\mathcal{N}$ for Gaussian density, $\mathcal{W}$ for the Weibull, $\mathcal{G}$ for the Gamma, $\mathcal{E}$ for the exponential, $\mathcal{E}r$ for the Erlang, $\mathcal{M}$ the double-sided Maxwell, and $\mathcal{P}$ for the Poisson. We always use $\theta$ to
denote the parameter the derivative triple applies to. }
    \label{fig:weak-derivatives}
\end{figure}

TODO: Also does not need the loss to be differentiable, but we evaluate it twice per sample. But it benefits from variance reduction is the same randomness is used for both evaluations. Beware it has a different validity than the other 2, need to check whether local-domination still needed/sufficient (seen as providing weak derivatives, the loss should be bounded and continuous, which seems a bit annoying. But there are generalizations, see https://www.jmlr.org/papers/volume21/19-346/19-346.pdf)

\subsection{Hybrid methods}

Instead of reparametrizing a distribution $P(\theta)$ as $g(\theta)_*\sample$, we can "weakly reparametrize" as $f(\theta)_*G(\theta)$, and apply the REPARAM trick for $f$ and the REINFORCE estimator for $G$.
In this setting, we will obtain 
\begin{equation}
    \label{eqn:hybrid_method}
    \grad_\theta\mbe_{p(x;\theta)}[f(x)]=\mbe_{p(\epsilon;\theta)}[\grad_\theta f(g(\epsilon;\theta))]+\mbe_{p(\epsilon;\theta)}[f(g(\epsilon;\theta))\grad_\theta log(p(\epsilon;\theta))]
\end{equation}

\noindent \textbf{Gamma Weak Reparameterisation}.
The Gamma distribution $\mathcal{G}(x;\alpha,\beta)$ can be represented as

\begin{align*}
    \epsilon = g^{-1}(x;\alpha,\beta)=\frac{log(x)-\psi(\alpha)+\log(\beta)}{\sqrt{\psi_1(\alpha)}} \\
    p(\epsilon;\alpha,\beta) = \frac{e^{\alpha\psi(\alpha)}\sqrt{\psi_1(\alpha)}}{\Gamma(\alpha)}exp(\epsilon\alpha\sqrt{\psi_1(\alpha)}-exp(\epsilon\sqrt{\psi_1(\alpha)}+\psi(\alpha)))
\end{align*}
where $\psi$ is the digamma function, and $\psi_1$ its derivative.

The terms in equation \ref{eqn:hybrid_method} can now be rewritten as
\[\mbe_{p_\theta(x)}[\grad_xf(x)l(g^{-1}(x;\theta);\theta)]+\mbe_{p_\theta(x)}[f(x)(\grad_xlog~p_\theta(x)l(g^{-1}(x;\theta);\theta) +\grad_\theta log~p_\theta(x)+u(g^{-1}(x;\theta);\theta))]\]
where $l(\epsilon;\theta):= \grad_\theta g(\epsilon;\theta)$ and $u(\epsilon;\theta):= \grad_\theta log |\grad_\epsilon g(\epsilon;\theta)|$.

% \begin{itemize}
%     \item rejection sampling method: might not be able to encode its condition as a higher-order function just yet
%     \item Generalized Pathwise Gradients and Stein-type Estimators (didn't really get this one)
%     \item Generalized Score Functions and Malliavin-weighted Estimators (uses Stein's identity again)
% \end{itemize}

In many statistical problems, the gradient of the entropy of a probabilistic model is an often required
informational quantity:
\[\grad_\theta \mathbb{H}[p(x;\theta)]=-\grad_\theta\mbe_{p(x;\theta)}[log~p(x;\theta)]\]
To apply the pathwise estimator, we must be able to differentiate the log-probability, which implies
that it must be known. This will not always be the case, and one common setting where this is encountered in machine learning is when using likelihood-free or implicit probabilistic models.
In such cases, the general strategy we take is to use a substitute function that fills the role of the unknown cost function, like the unknown log-probability, and that gives the gradient information we need. 
In this way, we can create a more general pathwise estimator that can be used when the gradient of the cost function is unknown, but that will reduce to the familiar pathwise estimator from Section 5 when it is. 
Stein’s identity gives us a general tool with which to do this.

\begin{figure}[H]
    \centering
\begin{tabular}{|l|l|l|l|}
\hline
    Construct  & One line summary & Section  \\ \hline
   $\baseline:\RR^*\to \pmonad\RR\to \eRR$ & Adds a baseline for variance reduction & \ref{sub:baseline} \\
     $\addcost:\RR\to\mathcal{WP}1$ & Accounting for Control Flow & \ref{sub:scg} \\
    $\reinforce_\sigma:D\sigma\to \pmonad\sigma$ & Density-Carrying distributions & \ref{sec:densities}\\
   %$\flipimportance$ & $\II\to\II\to \pmonad \RR$ & Primitive from Storchastic & \ref{sub:storchastic} \\ 
     $\leaveoneout_\sigma:\NN\to D\sigma\to \eRR$ & Estimator from Storchastic & \ref{sub:storchastic} \\ 
      $\smc_\sigma:(\text{List}~\sigma \to \RR_{\geq 0}) \to (\sigma \to D\,\sigma) \to$ & Differentiable particle filter  & \ref{sub:particle-filter} \\
       \qquad$(\text{List}~\sigma \to \eRR) \to \NN \to \NN \to \eRR$  & & \\
      $\importance:D\sigma\times D\sigma\to \pmonad\sigma $ & Internalized stop-gradient  & \ref{sub:stop-grad} \\
      $\gammaimplicit:\posreal\times\posreal\to \pmonad \RR$& Gradient via Implicit Differentiation & \ref{sub:implicit-diff} \\ 
   $\poissonweak:\posreal \to \pmonad \NN$ & Gradient via Weak Derivatives & \ref{sub:weak-deriv} \\
   %  && Gradient via Weak Reparametrization \\
     \hline
\end{tabular}
  \caption{Extending ADEV with new types, constructs, constants}
    \label{fig:recap-new-primitives}
\end{figure}
